# Supplementary material for: Semi-Supervised Contrastive Learning with Orthonormal Prototypes
Source: arXiv:2512.07880 source file (2025-11-27)
Supplement: Supplementary file 1 [file Appendix-Proof-2.tex]

\begin{proof}
At each step of gradient descent, every point \( \mathbf{x}_i \) moves toward the negative of the mean of the other points with a step size \( \eta \). Let the mean of all \( b \) points before the gradient descent step be
\(
\bm{\mu}^{(0)} := \frac{1}{b} \sum_{i=1}^{b} \mathbf{x}_i^{(0)}.
\)
The update rule for the \( i \)-th point is given by:
\[
\mathbf{x}_i^{(1)} = \mathbf{x}_i^{(0)} - \eta \frac{1}{b-1} \left( b \bm{\mu}^{(0)} - \mathbf{x}_i^{(0)} \right) = \left( 1 + \frac{\eta}{b-1} \right) \mathbf{x}_i^{(0)} - \eta \frac{b}{b-1} \bm{\mu}^{(0)}.
\]
After the update, each point \( \mathbf{x}_i^{(1)} \) is normalized to have unit norm, i.e., 
\(
\hat{\mathbf{x}}_i^{(1)} = \frac{\mathbf{x}_i^{(1)}}{\|\mathbf{x}_i^{(1)}\|}.
\)
The expected norm of any updated vector is calculated as:
\begin{align}
\mathbb{E}[\|\mathbf{x}_i^{(1)}\|^2] = \left( 1 + \frac{\eta}{b-1} \right)^2 \mathbb{E}\left[\|\mathbf{x}_i^{(0)}\|^2\right] &+ \eta^2 \left( \frac{b}{b-1} \right)^2 \mathbb{E}\left[\|\bm{\mu}^{(0)}\|^2\right] \nonumber \\
&- 2 \eta \frac{b}{b-1} \left( 1 + \frac{\eta}{b-1} \right) \mathbb{E}\left[\mathbf{x}_i^{(0)\top} \bm{\mu}^{(0)}\right].
\label{eq-totalexp}
\end{align}
Since \( \mathbf{x}_i^{(0)} \) is uniformly distributed on the surface of an \( m \)-dimensional unit ball, its covariance is 
\(
\text{Cov}(\mathbf{x}_i^{(0)}) = \frac{1}{m} \mathbf{I}_m.
\)
Therefore, the covariance of the mean is
\[
\text{Cov}(\bm{\mu}^{(0)}) = \text{Cov}\left( \frac{1}{b} \sum_{i=1}^{b} \mathbf{x}_i^{(0)} \right) = \frac{1}{b^2} \sum_{i=1}^{b} \text{Cov}(\mathbf{x}_i^{(0)}) = \frac{1}{bm} \mathbf{I}_m.
\]
The second moment of \( \bm{\mu}^{(0)} \)'s norm is the trace of its covariance matrix:
\begin{align}    
\mathbb{E}[\|\bm{\mu}^{(0)}\|^2] = \mathbb{E}[\bm{\mu}^{(0)\top} \bm{\mu}^{(0)}] = \text{Tr}(\text{Cov}(\bm{\mu}^{(0)})) = \frac{1}{bm} \text{Tr}(\mathbf{I}_m) = \frac{1}{b}.
\label{eq-2ndterm}
\end{align}
Since \( \mathbf{x}_i^{(0)} \) and \( \mathbf{x}_j^{(0)} \) are independent for \( i \neq j \), we know that \( \mathbb{E}[\mathbf{x}_i^{(0)\top} \mathbf{x}_j^{(0)}] = 0 \). Therefore, 
\begin{align}
    \mathbb{E}[\mathbf{x}_i^{(0)\top} \bm{\mu}^{(0)}] = \mathbb{E}\left[ \frac{1}{b} \|\mathbf{x}_i^{(0)}\|^2 + \frac{1}{b} \sum_{j \neq i} \mathbf{x}_i^{(0)\top} \mathbf{x}_j^{(0)} \right] = \frac{1}{b} \mathbb{E}[\|\mathbf{x}_i^{(0)}\|^2].
\label{eq-3rdterm}
\end{align}
Since \( \mathbb{E}[\|\mathbf{x}_i^{(0)}\|^2] = 1 \), substituting equations \eqref{eq-2ndterm} and \eqref{eq-3rdterm} into \eqref{eq-totalexp}, we obtain
\begin{align*}
\mathbb{E}[\|\mathbf{x}_i^{(1)}\|^2] &= \left( 1 + \frac{\eta}{b-1} \right)^2 +  \frac{b \eta^2}{(b-1)^2 } - 2 \eta \frac{b}{b-1} \left( 1 + \frac{\eta}{b-1} \right) \frac{1}{b} \\
&= 1 + \frac{\eta}{b-1} - \frac{2 \eta}{b}  - 2 \frac{\eta^2}{b(b-1)} + \frac{\eta^2 b}{(b-1)^2}.
\label{eq-2rd_exp}
\end{align*}
Thus, the upper bound of the first-order expectation \( \mathbb{E}[\|\mathbf{x}_i^{(1)}\|] \) can be denoted by \( B \), where:
\[
\mathbb{E}[\|\mathbf{x}_i^{(1)}\|] \leq \sqrt{1 + \frac{\eta}{b-1} - \frac{2 \eta}{b}  - 2 \frac{\eta^2}{b(b-1)} + \frac{\eta^2 b}{(b-1)^2}} := B.
\]
After the gradient descent step, the expectation of the new mean \( \bm{\mu}^{(1)} \) is bounded as follows:
\[
\bm{\mu}^{(1)} = \frac{1}{b} \sum_{i=1}^b \hat{\mathbf{x}}^{(1)}_i \geq \frac{1}{bB} \sum_{i=1}^b \mathbf{x}^{(1)}_i = \frac{1 - \eta}{B} \bm{\mu}^{(0)}.
\]
To prevent complete collapse in $\bm{\mu}^{(1)}$, the mean should not increase by more than $1 + \varepsilon$, where $\varepsilon$ controls the tolerance for mean shift. By setting $\varepsilon = 0$, we can ensure that $\bm{\mu}^{(1)}$ does not exceed $\bm{\mu}^{(0)}$, thereby providing the safest bound for the learning rate. This implies that the learning rate \( \eta \) must satisfy
\(
\frac{1 - \eta}{B} \leq 1 + \varepsilon.
\)
This gives the condition:
\[
(1 - \eta)^2 \leq \left( 1 + \frac{\eta}{b-1} - \frac{2 \eta}{b}  - 2 \frac{\eta^2}{b(b-1)} + \frac{\eta^2 b}{(b-1)^2} \right) (1+\varepsilon)^2.
\]

By setting $\varepsilon = 0$, we can simplify further to obtain the following inequality:
\[
\left(-2 - \frac{1}{b-1} + \frac{2}{b}\right) + \eta \left(1 + 2 \frac{1}{b(b-1)} - \frac{b}{(b-1)^2}\right) \leq 0.
\]
For \( b > 2 \), we have \( 1 + 2 \frac{1}{b(b-1)} - \frac{b}{(b-1)^2} > 0 \), leading to the bound:
\[
\eta \leq \frac{2 + \frac{1}{b-1} - \frac{2}{b}}{1 + 2 \frac{1}{b(b-1)} - \frac{b}{(b-1)^2}} = \frac{2b^3 - 5b^2 + 5b - 2}{b^3 - 3b^2 + 4b - 2} = 2 + O\left(\frac{1}{b}\right).
\]

Since $b$ is an integer, this bound is effectively $O(1 + \frac{1}{b})$.
\end{proof}
