# Supplementary material for: Semi-Supervised Contrastive Learning with Orthonormal Prototypes
Source: arXiv:2512.07880 source file (2025-11-27)
Supplement: Supplementary file 2 [file Appendix-Proof-3.tex]

\begin{proof}
Consider a list of \( k \) \textit{class embeddings} in \( m \)-dimensional space, denoted as \( \X := [\x_1, \dots, \x_k] \in \mathbb{R}^{m \times k} \), where \( m \geq k \) and each \textit{class embedding} has unit norm (i.e., \( \|\x_i\|_2 = 1 \) for all \( i \)). The loss function is defined as the sum of pairwise cosine similarities between the \textit{class embeddings} (refer to Equation~\ref{eq-total-cossim}).
We first assume that all \textit{class embeddings} are linearly independent, implying that \( \text{Rank}(\X) = k \). Our first goal is to show that there always exists another matrix \( \X' \in \mathbb{R}^{m \times k} \) with \( \text{Rank}(\X') = k-1 \), such that \( \mathcal{L}(\X) > \mathcal{L}(\X') \).

To construct such a matrix \( \X' \), we select a \textit{class embedding} \( \x_k \) such that \( \sum_{i \neq k} \x_i \neq 0 \). The existence of such a \textit{class embedding} \( \x_k \) can be easily established by contradiction. Suppose, for the sake of contradiction, that for all \( k \), \( \sum_{i \neq k} \x_i = 0 \). This would imply that each \( \x_i \) must be zero, i.e., \( \x_i = 0 \) for all \( i \), which contradicts the assumption that the $\text{Rank}(\X) = k$. Hence, such a \textit{class embedding} \( \x_k \) must exist.
Since the \textit{class embeddings} are linearly independent, \( \x_k \) can be decomposed as a weighted sum of two unit-norm vectors: one orthogonal to all other \textit{class embeddings}, and one lying in the subspace spanned by the remaining \textit{class embeddings}. Specifically, we write:
\[
\x_k = \eta \x_k^\perp + \sqrt{1 - \eta^2} \x_k^\parallel, \quad 0 < \eta \leq 1,
\]
where \( \x_k^\perp \) is orthogonal to all other \textit{class embeddings} and \( \x_k^\parallel \) lies in the subspace spanned by the remaining \textit{class embeddings}.
The loss associated with the \( k \)-th \textit{class embedding} is:
\[
\mathcal{L}_{k}(\X) = \sum_{i \neq k} \x_i^\top \x_k = \sum_{i \neq k} \x_i^\top \left( \eta \x_k^\perp + \sqrt{1 - \eta^2} \x_k^\parallel \right).
\]
Since \( \x_i^\top \x_k^\perp = 0 \) for all \( i \neq k \), we have:
\[
\mathcal{L}_{k}(\X) = \sqrt{1 - \eta^2} \sum_{i \neq k} \x_i^\top \x_k^\parallel.
\]
Now, construct \( \X' \) by replacing \( \x_k \) with \( \x_k^\parallel \). The corresponding loss function becomes:
\[
\mathcal{L}_{k}(\X') = \sum_{i \neq k} \x_i^\top \x_k^\parallel.
\]
It is important to note that we can always find \( \sum_{i \neq k} \x_i^\top \x_k^\parallel < 0 \). If this sum is not negative, we can simply invert the sign of \( \x_k^\parallel \), ensuring the sum becomes negative. 
Since \( 0 < \eta \leq 1 \), it follows that \( \sqrt{1 - \eta^2} < 1 \). Consequently,
$
\sqrt{1 - \eta^2} \sum_{i \neq k} \x_i^\top \x_k^\parallel >  \sum_{i \neq k} \x_i^\top \x_k^\parallel.
$
Therefore, we have \( \mathcal{L}(\X) > \mathcal{L}(\X') \), as required.
\end{proof}
