# Supplementary material for: Semi-Supervised Contrastive Learning with Orthonormal Prototypes
Source: arXiv:2512.07880 source file (2025-11-27)
Supplement: Supplementary file 3 [file Appendix-relatedwork.tex]

\begin{table*}[h]
\setlength{\tabcolsep}{0pt}
    \centering
    \begin{tabular}{l|ccc|cc}
        \hline
        Method   & Affinity Metric & Aff. to Prob. & Divergence Function & Top-1 & Top-5   \\ 
        \hline
         CPC-v2 \cite{henaff2020data} & Cosine & Softmax &CrossEntropy &   71.5 & 90.1 \\
         MOCO-v2 \cite{chen2020improved} &Cosine & Softmax &CrossEntropy  & 71.1 & - \\ 
         SimCLR \cite{chen2020simple} &Cosine & Softmax &CrossEntropy  &69.3 & 89.0 \\
         \hline
        \multicolumn{6}{c}{Inclusion/Removal of Terms within InfoNCE} \\ 
        \hline
         PCL \cite{cui2021parametric} &Cosine & Softmax &CrossEntropy & 67.6 & -\\
         LOOC \cite{xiao2020should} & Cosine & Softmax & CrossEntropy Variant & - & -\\
         DCL  \cite{yeh2022decoupled}& Cosine & Decoupled Sftmx & CrossEntropy  & 68.2 & -\\
         RC  \cite{wang2022rethinking} & Cosine & Softmax & CrossEntropy +  L2 & 61.6 & - \\ 
         \hline
         \multicolumn{6}{c}{Adjustments to the Similarity Function of InfoNCE}         \\ 
         \hline
         Debiased \cite{chuang2020debiased} & Floor Cosine & Softmax & CrossEntropy & - & - \\
         GCL \cite{koishekenov2023geometric} & Arccosine &  Softmax & CrossEntropy & - & - \\ 
         HCL  \cite{ge2023hyperbolic} & Cos. + Poincar\'e &  Softmax & CrossEntropy & 58.5 & - \\ 
         \hline
         \multicolumn{6}{c}{Innovations}         \\ \hline
         InfoMin \cite{tian2020makes} &Cosine & Softmax & MinMax CrossEntropy & \textbf{73.0} & 91.1\\
         VICref \cite{bardes2021vicreg} &Euclidean & NA &Distance + Var + Cov  & \textbf{73.1} & 91.1\\
         BT \cite{zbontar2021barlow} &Dimensional Cos.& NA & L2 & \textbf{73.2} & 91.0 \\
        \hline
    \end{tabular}
    \caption{Overview of Novel Loss Functions and Baseline Results from 2020: Image Classification Accuracy on ImageNet1K with Unsupervised Learning and Full Label Fine-Tuning. The accuracy measurements are based on training a standard ResNet-50 with 24M parameters. The symbol '-' indicates that the corresponding metric was not reported in the original paper.}
    \label{tab:unsup}
\end{table*}
